# Supplementary material for: Online Detection of Sparse Changes in High-Dimensional Data Streams Using Tailored Projections
Source: arXiv:1908.02029 source file (2019-08-06)
Supplement: Supplementary file 1 [file 2dProofs.tex]

\documentclass[a4paper, english, 11pt]{article}
\usepackage[utf8]{inputenc}

\input{C:/Users/matve/OneDrive/Dokumenter/Studier/PhD/LatexSetup}
\input{C:/Users/matve/OneDrive/Dokumenter/Studier/PhD/LatexCommands}

\usepackage[margin=1in]{geometry}

\def\spacingset#1{\renewcommand{\baselinestretch}%
{#1}\small\normalsize} \spacingset{1}
\spacingset{1.45} % DON'T change the spacing! (Double spaced)
%opening

\begin{document}
\subsection{Proofs of the two-dimensional propositions} \label{sec:A_proofs}

Before turning to the the proofs of the propositions in section \ref{sec:2},
the expressions for the pre- and post-change means and variances of each projection is needed.
The normalized eigenvectors (principal axes) and corresponding eigenvalues (variance in the data along a given principal axis) of 
$\bSigma_0$ are quickly verified to be
\begin{equation}
\begin{split}
&\lambda_1 = 1 + \rho, \quad
\mathbf{v}_1 = \frac{1}{\sqrt{2}}
\begin{pmatrix}
1 \\
1
\end{pmatrix} \\
&\lambda_2 = 1 - \rho, \quad
\mathbf{v}_2 = \frac{1}{\sqrt{2}}
\begin{pmatrix}
-1 \\
1
\end{pmatrix}
\end{split}
\label{eq:eigenSpace}
\end{equation}
Note that which principal axis is the dominant one depends on the sign of $\rho$.
If $\rho$ is positive, $\mathbf{v}_1$ is the dominant one, but $\mathbf{v}_2$ is dominant if $\rho$ is negative.

From the given projections in \eqref{eq:eigenSpace}, the variances of the projections can be expressed as functions of the original correlation matrix and multiplicative change factors.
Recall that we write the post-change covariance matrix as
\[
  \bSigma_1 = 
  \begin{pmatrix}
    a_{11}^2 & a_{11}a_{22}a_{12}\rho \\
    a_{11}a_{22}a_{12}\rho & a_{22}^2
  \end{pmatrix}.
\]
where $a_{11}, a_{22} > 0$ and 
\begin{equation}
  -1 < a_{12} \rho < 1.
  \label{eq:corBound}
\end{equation}
The original and changed variances of the most varying principal component can then be written as follows, respectively.
\begin{equation}
\begin{split}
o_1^2 &= 1 + \rho \\
c_1^2 &= \frac{1}{2}a_{11}^2 + \frac{1}{2}a_{22}^2 + a_{11}a_{22}a_{12}\rho.
\end{split}
\label{eq:topPCvariances}
\end{equation}
Moreover, the expressions for the variances along the least varying principal axes are identical up to one switched sign,
\begin{equation}
\begin{split}
o_2^2 &= 1 - \rho \\
c_2^2 &= \frac{1}{2}a_{11}^2 + \frac{1}{2}a_{22}^2 - a_{11}a_{22}a_{12}\rho.
\end{split}
\label{eq:botPCvariances}
\end{equation}
Observe that if $\rho < 0$, then $o_2$ and $c_2$ would be equal to $o_1$ and $c_1$ with positive $\rho$, and vice versa.
Thus, for $\rho \in (-1, 1)$, the general expressions are obtained by replacing $\rho$ with $|\rho|$.

Finally, the changed mean components are given by
\begin{equation}
\begin{split}
m_1 &= \frac{1}{\sqrt{2}}(\mu_{1} + \mu_{2}) \\
m_2 &= \frac{1}{\sqrt{2}}(\mu_{1} - \mu_{2}).
\end{split}
\label{eq:PCmeans}
\end{equation}

We first prove the proposition for changes in the mean. It is restated below for completeness.
\begin{myprop} \label{prop:mean}
  Let $a_{11} = a_{22} = a_{12} = 1$ (constant covariance matrix).
  $H_2 > H_1$ if and only if $(\mu_1 - \mu_2)^2 > \mu_1\mu_2 (4/|\rho| - 2)$.
  In particular, for $|\rho| \in (0, 1)$,
  \begin{enumerate}[label=(\roman*)]
    \item $H_2 > H_1$ if one of $\mu_1$ and $\mu_2$ is $0$ while the other is not (one mean changes).
    \item $H_2 > H_1$ if $\mu_1 = -\mu_2 = \mu \not= 0$ (equal changes in opposite directions).
    \item $H_2 < H_1$ if $\mu_1 = \mu_2 = \mu \not= 0$ (equal changes in the same direction).
  \end{enumerate}
\end{myprop}
\begin{proof}[Proof of Proposition \ref{prop:mean}]
Let $p_1(x) = N(x | 0, o_1^2)$, $q_1(x) = N(x | m_1, o_1^2)$,
$p_2(x) = N(x | 0, o_2^2)$ and $q_2(x) = N(x | m_2, o_2^2)$, where $m_i, o_i$ are as in \eqref{eq:topPCvariances}, \eqref{eq:botPCvariances} and \eqref{eq:PCmeans}, with $\rho$ replaced by $|\rho|$ as noted above.
The Hellinger distances between the distributions before and after a change along each principal axis is given by
\[
  H_j^2 = H^2(p_j, q_j) = 1 - \exp\left\{ - \frac{1}{8o_j^2}m_j^2 \right\}.
\]
Then some algebra results in the inequality we needed to prove;
\begin{align*}
  H_2 &> H_1 \\
  (1 + |\rho|)(\mu_1 - \mu_2)^2 &> (1 - |\rho|)(\mu_1 + \mu_2)^2 \\
  |\rho| (\mu_1 - \mu_2)^2 + \mu_1\mu_2(2|\rho| - 4) &> 0 \\
  (\mu_1 - \mu_2)^2 &> \mu_1\mu_2 (4/|\rho| - 2).
\end{align*}
From this inequality, the three special cases (i), (ii) and (iii) are immediately given.
\end{proof}

In the proofs concerning changes in the covariance matrix, we will make use of the following lemma.
It reduces the inequality of Hellinger distances to a simpler inequality of ratios of variances.
\begin{mylemma} \label{lem:HellingerEquiv}
  Let $p_1, q_1, p_2, q_2$ be 0-mean normal distribution functions with variances $\sigma^2_{p_1}, \sigma^2_{q_1}, \sigma^2_{p_2}$ and $\sigma^2_{q_2}$, respectively.
  Furthermore, let
  \[
    \log r_j = \left|\log \frac{\sigma^2_{q_j}}{\sigma^2_{p_j}}\right|, \quad j = 1, 2.
  \]
  Then $H(p_2, q_2) > H(p_1, q_1)$ if and only if $\log r_2 > \log r_1$.
\end{mylemma}
\begin{proof}
  First observe that when the means are $0$ we can write the Hellinger distance between two normal distributions as the following.
  \begin{align*}
    H^2 (p, q) &= 1 - \left( \frac{2\sigma_p\sigma_q}{\sigma_p^2 + \sigma_q^2} \right)^{1/2} \\
    &= 1 - \sqrt{2}\left( \frac{\sigma_p}{\sigma_q} + \frac{\sigma_q}{\sigma_p} \right)^{-1/2} \\
    &= 1 - \sqrt{2}\left( \frac{\sigma_p^2}{\sigma_q^2} + \frac{\sigma_q^2}{\sigma_p^2} + 2 \right)^{-1/4}.
  \end{align*}
  This gives us the inequality
  \begin{align*}
    H(p_2, q_2) &> H(p_1, q_1) \\
    \frac{\sigma_{p_2}^2}{\sigma_{q_2}^2} + \frac{\sigma_{q_2}^2}{\sigma_{p_2}^2} &> \frac{\sigma_{p_1}^2}{\sigma_{q_1}^2} + \frac{\sigma_{q_1}^2}{\sigma_{p_1}^2}.
  \end{align*}
  By setting $r_2 = \sigma_{p_2}^2 / \sigma_{q_2}^2$ and $r_1 = \sigma_{p_1}^2 / \sigma_{q_1}^2$, the inequality can be written as
  \[
    r_2 + r_2^{-1} > r_1 + r_1^{-1}.
  \]
  Now assume first that $r_1, r_2 > 1$, i.e., $\sigma_{p_j}^2 > \sigma_{q_j}^2$.
  Then we see that
  \begin{align*}
    r_2 + r_2^{-1} &> r_1 + r_1^{-1} \\
    r_2 - r_1 + \frac{r_1 - r_2}{r_1r_2} &> 0 \\
    (r_2 - r_1)\Big(1 - \frac{1}{r_1r_2}\Big) &> 0.
  \end{align*}
  By the assumption that $r_1, r_2 > 1$, this inequality holds if and only if $r_2 > r_1$.
  
  Finally, note that by interchanging $\sigma_{p_j}^2$ and $\sigma_{q_j}^2$, the same result is obtained when $\sigma_{q_j}^2 \geq \sigma_{p_j}^2$.
  Thus, to make the result hold in general, we can set
  \[
    r_j = \exp\left\{\Big|\log \frac{\sigma^2_{q_j}}{\sigma^2_{p_j}}\Big|\right\}, \quad j = 1, 2,
  \]
  which is an expression for the ratio between variances where the largest of the variances is always in the numerator.
  Therefore we get that $\log r_2 > \log r_1$ is equivalent to $H_2 > H_1$.
\end{proof}

\begin{myprop} \label{prop:2var}
  Let $\mu_1 = \mu_2 = 0$, $a_{12} = 1$ and $a_{11} = a_{22} = a \not= 1$ (both variances change equally).
  For any $|\rho| \in (0, 1)$ and $a > 0$, $H_2 = H_1$.
\end{myprop}

\begin{proof}[Proof of Proposition \ref{prop:2var}]
When assuming that $a_{12} = 1$ and $a_{11} = a_{22} = a \not= 1$, we get that
\[
  \log r_2 = \left| \log \frac{a^2/2 + a^2/2 - |\rho| a^2}{1 - |\rho|} \right| = |\log a^2|,
\]
and
\[
  \log r_1 = \left| \log \frac{a^2/2 + a^2/2 + |\rho| a^2}{1 + |\rho|} \right| = |\log a^2|.
\]
Hence, by arguments similar to the proof of Lemma \ref{lem:HellingerEquiv}, we see that $H_2 = H_1$ no matter what $|\rho|$ or $a$ is.
\end{proof}

\begin{myprop} \label{prop:1var}
  Let $\mu_1 = \mu_2 = 0$, $a_{12} = 1$, and either $a_{11} = 1$ and $a_{22} = a \not= 1$, or $a_{11} = a$ and $a_{22} = 1$, where $a > 0$ (one variance changes).
  \begin{enumerate}[label=(\roman*)]
    \item For any $|\rho| \in (0, 1)$ and $a > 1$ (variance increase), $H_2 > H_1$.
    %\item When $0 < a < 1$ (variance decrease) and $|\rho| < \sqrt{3}/2$, $H_1 > H_2$.
    %$H_1 > H_2$ also holds when $|\rho| > \sqrt{3}/2$ and $a > \sqrt{2\rho^2 - 1}$.
    %However, $H_2 > H_1$ if $|\rho| > \sqrt{3}/2$ and ${0 \leq a \leq \sqrt{2\rho^2 - 1}}$.
    \item When $|\rho| \in (0, 1)$ and $a \in (0, 1)$ (variance decrease), $H_2 < H_1$ in most cases. 
    The only exception is if $|\rho| \in (\sqrt{3}/2, 1)$ and $a \in (0, \sqrt{4\rho^2 - 3})$, where $H_2 > H_1$.
  \end{enumerate}
\end{myprop}
\begin{proof}[Proof of Proposition \ref{prop:1var}]
  Using the formulas for the variances of the projections \eqref{eq:topPCvariances} and \eqref{eq:botPCvariances},
  the inequality we have to study according to Lemma \ref{lem:HellingerEquiv} becomes the following,
  \begin{align}
    \left| \log \frac{a^2 - 2a|\rho| + 1}{2(1 - |\rho|)} \right| &> \left| \log \frac{a^2 + 2a|\rho| + 1}{2(1 + |\rho|)} \right| \notag \\
    \left| \log \left[ \frac{(1 - a)^2}{2(1 - |\rho|)} + a \right] \right| &> \left| \log \left[ \frac{(1 - a)^2}{2(1 + |\rho|)} + a \right] \right|. \label{eq:1var_ineq}
  \end{align}
  First, we have to find out the sign of the expressions inside the absolute values for each $a$ and $|\rho|$.
  For the left-hand side, we get
  \begin{align*}
    &\frac{(1 - a)^2}{2(1 - |\rho|)} + a = 1 \\
    &a = 1 \text{ and } a = 2|\rho| - 1.
  \end{align*}
  Thus, for $a > 1$ and $a < 2|\rho| - 1$, the left-hand side is positive, while negative in between.
  For the right-hand side, the expression inside the absolute value signs are positive for $a > 1$ and $a < - (1 + 2|\rho|)$. 
  Since $a > 0$, however, the relevant root for the right-hand side is only $a = 1$.
  In total, this gives us three regions of $(a, |\rho|)$-values to check inequality \eqref{eq:1var_ineq}: $a > 1$ and $|\rho| \in (0, 1)$, $a \in (2|\rho| - 1, 1)$ and $|\rho| \in (0, 1)$, and $a \in (0, 2|\rho| - 1)$ and $|\rho| \in (1/2, 1)$.
  \paragraph{$a > 1$ and $|\rho| \in (0, 1)$:}
  The absolute value signs can now be dissolved, so that inequality \eqref{eq:1var_ineq} becomes
  \[
    \frac{(1 - a)^2}{(1 - |\rho|)} > \frac{(1 - a)^2}{(1 + |\rho|)}.
  \]
  Since $|\rho| \in (0, 1)$, we see that the inequality holds for any $a > 1$.
  Hence, $H_2 > H_1$ in this scenarios, when the variance increases.
  \paragraph{$a \in (2|\rho| - 1, 1)$ and $|\rho| \in (0, 1)$:}
  In this case, inequality \eqref{eq:1var_ineq} becomes
  \[
    \frac{(1 - a)^2}{(1 - |\rho|)} < \frac{(1 - a)^2}{(1 + |\rho|)}.
  \]
  I.e., it does not hold for any of the $a$'s or $|\rho|$'s within the relevant region. Note that when $|\rho| < 1/2$, $a$ is kept between $(0, 1)$.
  \paragraph{$a \in (0, 2|\rho| - 1)$ and $|\rho| \in (1/2, 1)$:}
  Now we get the inequality
  \[
    \frac{(1 - a)^2}{2(1 - |\rho|)} + a > \left(\frac{(1 - a)^2}{2(1 + |\rho|)} + a\right)^{-1},
  \]
  which is equivalent to
  \begin{equation}
    a^4 - a^2(4\rho^2 - 2) + 4\rho^2 - 3 > 0.
    \label{eq:1var_tedious}
  \end{equation}
  The roots of the function on the left-hand side are $a = \pm 1$ and $a = \pm \sqrt{4\rho^2 - 3}$, but the only relevant root for $a \in (0, 2|\rho| - 1)$ and $|\rho| \in (1/2, 1)$ is $a_0 := \sqrt{4\rho^2 - 3}$.
  
  Next, for $|\rho| < \sqrt{3}/2$ the root $a_0$ moves into the complex plane, and the function on the left-hand side of \eqref{eq:1var_tedious} is always less than $0$ for the relevant $a$'s. I.e., $H_2 < H_1$ in this case.
  If $|\rho| > \sqrt{3}/2$, on the other hand, then \eqref{eq:1var_tedious} holds for $a \in (0, a_0)$, but not for $a \in (a_0, 2|\rho| - 1)$.
\end{proof}

\begin{myprop} \label{prop:cor}
  Let $\mu_1 = \mu_2 = 0$, $a_{11} = a_{22} = 1$ and $a_{12} = a \not= 1$ such that \eqref{eq:corBound} holds.
  Then $H_2 > H_1$ for any $|\rho| \in (0, 1)$ and $a > -1$.
\end{myprop}
\begin{proof}[Proof of Proposition \ref{prop:cor}]
  In this scenario, the inequality to check due to Lemma \ref{lem:HellingerEquiv} and expressions \eqref{eq:topPCvariances} and \eqref{eq:botPCvariances} is
  \begin{equation}
    \left| \log \frac{1 - a|\rho|}{1 - |\rho|} \right| > \left| \log \frac{1 + a|\rho|}{1 + |\rho|} \right|.
    \label{eq:cor_ineq}
  \end{equation}
  To dissolve the absolute value signs we first have to see for which values of $a$ and $|\rho|$ the expressions inside are positive or negative. It is easily verified that the expression inside the left-hand side absolute value is positive for $a < 1$, while the right-hand side is positive if $a > 1$, both being negative otherwise.
  
  First assume that $a < 1$. Then inequality \eqref{eq:cor_ineq} becomes 
  \begin{align*}
    \frac{1 - a|\rho|}{1 - |\rho|} &> \frac{1 + |\rho|}{1 + a|\rho|} \\
    1 - (a\rho)^2 &> 1 - \rho^2 \\
    a^2 &< 1
  \end{align*}
  Hence, $a \in (-1, 1)$ yields $H_2 > H_1$.
  On the other hand, if $a > 1$, we obtain
  \begin{align*}
    \frac{1 - |\rho|}{1 - a|\rho|} &> \frac{1 + a|\rho|}{1 + |\rho|} \\
    a^2 &> 1,
  \end{align*}
  which is always true.
  Thus, in total, $H_2 < H_1$ only if $a < -1$.
\end{proof}

\end{document}
